# Supplementary material for: Learning to Deceive Knowledge Graph Augmented Models via Targeted Perturbation
Source: arXiv:2010.12872 source file (2021-05-03)
Supplement: Supplementary file 1 [file 9_appendix.tex]

% !TEX root = main.tex

\section{Appendix}
You may include other additional sections here.
